# Supplementary material for: Large Language Models as Source Planner for Personalized Knowledge-grounded Dialogue
Source: arXiv:2310.08840 source file (2023-10-13)
Supplement: Supplementary file 1 [file ablation_nli.tex]

\begin{table}[!t]
    \centering
    \begin{adjustbox}{max width=0.48\textwidth}
    \begin{tabular}{l|c|c}
    \toprule
    \textbf{Model} & \hspace{0.5cm} \textbf{P.NLI} \hspace{0.5cm} & \hspace{0.5cm} \textbf{K.NLI} \hspace{0.5cm} \\
    % \hline
    % \hline
    % \multicolumn{5}{c}{\textit{\textbf{Supervised}}} \\
    \hline
    \hline
    \textsc{chatglm-6b} & 85.77 (991) & 44.42 (840) \\
    \hdashline
    \quad + Ground Planning & 83.78 (1048) & 42.90 (923) \\
    \quad + Ground Retrieval & 88.39 (999) & 62.02 (853) \\
    \quad + Ground P \& R & \textbf{88.93} (1048) & \textbf{64.03} (923) \\
    \hdashline
    \quad - Dependency & 82.91 (1002) & 42.33 (851) \\
    \quad - Documents & 85.49 (1006) & 38.03 (852) \\
    \quad - Planning$^*$ & 87.69 (1048) & 49.72 (923) \\
    \bottomrule
    \end{tabular}
    \end{adjustbox}
    \caption{The NLI performance of different steps and modules in the SAFARI framework.}
    \label{tab:abla_nli}
\end{table}
