# Supplementary material for: Large Language Models as Source Planner for Personalized Knowledge-grounded Dialogue
Source: arXiv:2310.08840 source file (2023-10-13)
Supplement: Supplementary file 2 [file minda_c.tex]

\begin{table}[!t]
    \centering
    \begin{adjustbox}{max width=0.48\textwidth}
    \begin{tabular}{l|c|c|c|c}
    \toprule
    \textbf{Model} & \textbf{BLEU1} & \textbf{RougeL} & \textbf{P.C} & \textbf{K.C} \\
    % \hline
    % \hline
    % \multicolumn{5}{c}{\textit{\textbf{Supervised}}} \\
    \hline
    \hline
    \textsc{chatglm-6b} & 23.81 & 26.70 & 80.63 & 54.03 \\
    \hdashline
    \quad + Ground Planning & 24.29 & 27.01 &  \\
    \quad + Ground Retrieval & \textbf{25.86} & 29.15 &  \\
    \quad + Ground P \& R & 25.71 & \textbf{29.43} &  \\
    \hdashline
    \quad - Dependency & 23.32 & 26.53 & \\
    \quad - Documents & \underline{23.06} & \underline{25.34} & \\
    \quad - Planning$^*$ & 25.31 & 28.77 & 78.68 & 55.89 \\
    % \quad - P \& R & 26.12 & 27.71 & 76.71 & 30.98 \\
    % \multicolumn{5}{c}{\textit{\textbf{Unsupervised}}} \\
    % \hline
    % \hline
    % \textsc{chatgpt} & \\
    % \hdashline
    % \quad + Ground Planning \\
    % \quad + Ground Retrieval \\
    % \quad + Both \\
    \bottomrule
    \end{tabular}
    \end{adjustbox}
    \caption{The performance (minda.C) of different steps and modules in SAFARI framework. $^*$ means that the model is re-trained.}
    \label{tab:minda_c}
\end{table}
