# Supplementary material for: Large Language Models as Source Planner for Personalized Knowledge-grounded Dialogue
Source: arXiv:2310.08840 source file (2023-10-13)
Supplement: Supplementary file 3 [file not_calibrated_nli.tex]

\begin{table}[!t]
    \centering
    \begin{adjustbox}{max width=0.48\textwidth}
    \begin{tabular}{l|c|c}
    \toprule
    \textbf{Model} & \hspace{0.5cm} \textbf{P.NLI}\hspace{0.5cm} & \hspace{0.5cm}\textbf{K.NLI}\hspace{0.5cm} \\
    \hline
    \hline
    \multicolumn{3}{c}{\textit{\textbf{Supervised Setting}}} \\
    \hline
    \hline
    \textsc{belle-llama-7b-2m} & 90.58 (934) & 58.06 (813) \\
    \hline
    \textsc{chatglm-6b} & 85.77 (991) & 44.42 (840) \\
    \hline
    \hline
    \multicolumn{3}{c}{\textit{\textbf{Unsupervised Setting}}} \\
    \hline
    \hline
    \textit{Zero-shot} \\
    \textsc{belle-llama-7b-2m} & 80.59 (268) & 40.96 (188) \\
    \textsc{chatglm-6b} & 33.33 (3) & 0.0 (2) \\
    \textsc{chatgpt} & 93.36 (949) & 54.22 (675) \\

    \hline
    \textit{In-context} \\
    \textsc{belle-llama-7b-2m} & 86.79 (1022) & 0.0 (0)   \\
    \textsc{chatglm-6b} & 94.11 (34) & 36.36 (22) \\
    \textsc{chatgpt} & 94.71 (472) & 65.88 (255) \\

    \bottomrule
    \end{tabular}
    \end{adjustbox}
    \caption{The uncalibrated NLI performance of \textbf{Assembly} under supervised/unsupervised settings. We also report the frequency in the bracket.}
    \label{tab:appendix_no_calibrated_nli}
\end{table}
